# Supplementary material for: Adversarial Math Word Problem Generation
Source: arXiv:2402.17916 source file (2024-06-15)
Supplement: Supplementary file 1 [file difficult_pro_4_model.tex]

\section{Shared Attacks}\label{difficult_pro_4_model}
In this section we investigate whether given some problems, can we quickly find what are the subset of problems that GPT-4 tends to fail. Given the problem transferability among the models in Figure \ref{fig:transferability}, we first check whether these models share the same correctly solved problems with GPT-4. We randomly select 5 problems that models make correct predictions for, along with their 100 adversarial examples in GSM8K M3, and test them with GPT-4. Note that for some models, there are no correct responses, even with M3, the most subtle modifications. 

We report the model's performance that has correct predictions under Table \ref{table:share_attack} in the \textit{Shared Correct} column. We observe that GPT-4 aces all correct problems from these models, which suggests GPT-4 and the other models have a strong alignment in correctly solving the same set of problems. Next, we perform the opposite, where we select the top 5 problems that have the highest number of adversarial examples that the model has failed and test them with GPT-4. Table \ref{table:efficient_attack} in the \textit{Shared Incorrect} column shows the result. We observe that the stronger models have higher degrees of shared incorrectness among the models and GPT-4 compared to the weaker models. This phenomenon suggests that using a stronger model to filter adversarial examples can be a cost-effective way to 
quickly identify what are the subset of problems that GPT-4 tends to fail. 

\begin{table}[ht!]
  \small
    \centering
  \begin{tabular}{lcc}
    \toprule
    \textbf{Model} & \textbf{Shared Correct} & \textbf{Shared Incorrect}  \\
    \midrule
    % Mistral 7B &  100 &  0  \\
    MetaMath 7B &  100 &  20    \\
    % Llama-2 13B &  100 &  0  \\
    WizardMath 13B & 100  &  40  \\
    % Vicuna 13B &  100 &  0 \\
    % CodeLlama 34B & 100  &  0   \\
    MetaMath 70B &  100 & 40   \\
    GPT-3.5-Turbo &  100 &  60    \\
    \bottomrule
  \end{tabular}
    \caption{\textbf{Quick Vulnerability Identification:} we present the shared correct and incorrect problems between models and GPT-4. All 100\% of shared correctness suggests GPT-4 has a strong alignment in correctly solving the same set of problems with other models. A different degree of shared incorrectness suggests that the strong models have similar vulnerabilities to certain adversarial examples with GPT-4, which can be effectively used to undermine GPT-4's performance with lower computational cost.}
  \label{table:efficient_attack}
  \vspace{-1em}
\end{table}
