# Supplementary material for: Adversarial Math Word Problem Generation
Source: arXiv:2402.17916 source file (2024-06-15)
Supplement: Supplementary file 2 [file node_property_detail.tex]

\section{Node properties} \label{appendix:node_property_detail} \todo{need to be reworked}
For each node in the problem-solving tree, a set of properties is determined based on the original value $v$ of the node. A newly generated problem is valid if all nodes satisfy all desired properties. Let $v'$ be the new value of the node in a newly generated problem. Currently, four properties are stored for each node: \begin{enumerate}
    \item \textbf{Is positive}: this property is set to true if the value is strictly positive. The corresponding node in a newly generated problem will not satisfy this property only if $v$ is positive while $v'$ is not positive. If $v$ is not positive, then $v'$ can be any number and still satisfies this property.
    \item \textbf{Is an integer}: this property is set to true if the value is an integer; more specifically, this property is determined by $\code{abs(v - round(v')) <= 10^{-9}}$, meaning that a floating point number can still be considered an integer. Similar to the ``is positive'' property, the corresponding node in a newly generated problem will not satisfy this property only if $v$ is an integer while $v'$ is not an integer.
    \item \textbf{Number of digits}: this property is an integer that counts the number of prime factors that $v$ has; if $v$ doesn't satisfy the property ``is an integer'', then the number of factors is set to zero. Let $f(v)$ be the number of factors of $v$. The corresponding node in a newly generated problem satisfies this property if $f(v) \le f(v') + 1$ or $f(v')\ge 3$. The motivation for having this property is that numbers with more factors are usually ``easier" to work with, especially when the generated numbers will stay close to the original number. An example would be the number $135$ and the number $157$. Furthermore, some numbers have a high number of factors, that other numbers in their surroundings don't have; therefore, the newly generated number only needs to satisfy one of the two constraints. For example, the number $64$ has $6$ prime factors, while only $6$ numbers between 1 and 100 have prime factor counts more than 5. On the contrary, there are 40 numbers between 1 and 100 that have prime factor counts equal to or more than 3. 
    \item \textbf{Number of scientific numbers}: this property is an integer that counts the number of scientific integers in $v$ up to six decimal places. Let $s(v)$ be the number of scientific numbers in $v$. The corresponding node in a newly generated problem satisfies this property if $s(v)\ge s(v') - 1$. The motivation for preserving this property is that larger numbers don't usually make calculations harder, but more scientific numbers usually will make calculations harder. An example would be the number $150,000$ and the number $172,568$. 
\end{enumerate}
