# Supplementary material for: Adversarial Math Word Problem Generation
Source: arXiv:2402.17916 source file (2024-06-15)
Supplement: Supplementary file 3 [file universal_attack.tex]

\section{Universal Attack Results}  \label{appendix:universal_attack}
\begin{table}[ht!]
\small
\centering
\begin{tabular}{lrrrrr}
\toprule
\textbf{Model} & \textbf{Ct.} & $\textbf{M3}$ \textit{{(\%)}}& $\textbf{M2}$ \textit{{(\%)}} & $\textbf{M1}$ \textit{{(\%)}} \\
\midrule
Mistral 7B& 1 & 100.0 & 100.0 & 100.0\\
MetaMath 7B & 2& 70.0 & 90.0 & 100.0 \\
Llama 2 13B & 3& 67.0 & 90.0 & 100.0 \\
WizardMath 13B & 4& 52.0 & 80.0 & 100.0 \\
Vicuna 13B & 5& 44.0 & 78.0 & 100.0 \\
CodeLlama 34B & 6& 21.0 & 67.0 & 99.0 \\
MetaMath 70B & 7& 9.0 & 49.0 & 87.0 \\
GPT-3.5 & 8& 9.0 & 46.0 & 83.0 \\
\bottomrule
\end{tabular}
\caption{\textbf{Universal Attack:} All models share some percentage of universal attacks, implying that diversity among models could enhance resilience against such attacks.}
\label{table:universal_attack}
\vspace{1em}
\end{table}
