# Supplementary material for: Adversarial Math Word Problem Generation
Source: arXiv:2402.17916 source file (2024-06-15)
Supplement: Supplementary file 4 [file variable_grounding_example.tex]

\section{Variable Grounding Example} \label{appendix:variable_grounding_example}
Assume that we were given the question ``Mary and Ann are going sledding. Mary slides down a hill that's 630 feet long at a speed of 90 feet/minute. Ann slides down a hill that's 800 feet long at a rate of 40 feet/minute. How much longer does Ann's trip take than Mary?''. The corresponding code generated by GPT-4 and its problem-solving tree is shown in Figure \ref{fig:code}. Given that the numbers $(630, 90, 800, 40)$ both appeared in the original problem and the code, all nodes associated with the numbers are variable nodes. The binary operation node ``Ann Time'' has the operation divide and two children ``Ann Hill Length'' and ``Ann Speed''; its intermediate value is $20.0$, which will be used to determine the desired properties that the newly generated problem should have in this node. When the visitor visits the final print statement, its first argument $\code{int(time\_difference)}$ will be designated as the final answer. The expression $\code{int(time\_difference)}$ is a unary operation node with operation $\code{int}$ and operand $\code{time\_difference}$.
